# Supplementary material for: Role of Morphogenetic Competency on Evolution
Source: arXiv:2310.09318 source file (2023-10-13)
Supplement: Supplementary file 1 [file AppendixTemplate.tex]

% Appendix Template

\chapter{Appendix Title Here} % Main appendix title

\label{AppendixX} % Change X to a consecutive letter; for referencing this appendix elsewhere, use \ref{AppendixX}

Write your Appendix content here.
